# Supplementary material for: Towards GW Calculations on Thousands of Atoms
Source: arXiv:2104.09857 ancillary file (2021-04-20)
Supplement: Supplementary file 1 [file SuppInfo.pdf]

# Supporting Information for "Towards *GW* Calculations on Thousands of Atoms"

Jan Wilhelm,[1,*] Dorothea Golze,[2] Leopold Talirz,[3,4] Jürg Hutter,[1] and Carlo A. Pignedoli[5,†]

[1]*Department of Chemistry, University of Zurich, Winterthurerstrasse 190, CH-8057 Zurich, Switzerland*
[2]*COMP/Department of Applied Physics, Aalto University, P.O. Box 11100, FI-00076 Aalto, Finland*
[3]*Theory and Simulation of Materials, École Polytechnique Fédérale de Lausanne, Station 9, CH-1015 Lausanne, Switzerland*
[4]*Laboratory of Molecular Simulation, École Polytechnique Fédérale de Lausanne, Rue de l'Industrie 17, CH-1951 Sion, Switzerland*
[5]*Swiss Federal Laboratories for Materials Science and Technology (EMPA), Überlandstrasse 129, CH-8600 Dübendorf, Switzerland*

**CONTENTS**

I. Low-scaling vs. canonical *GW* algorithm in a Gaussian basis S2

II. Resolution of the identity S2

III. *GW*100 benchmark S3

IV. Outliers in the *GW*100 test set S5

V. Choosing the filter threshold S5

VI. Exemplary CP2K input file S6

VII. Basis sets for GNR benchmarks S7

VIII. References S8

## I. LOW-SCALING VS. CANONICAL *GW* ALGORITHM IN A GAUSSIAN BASIS

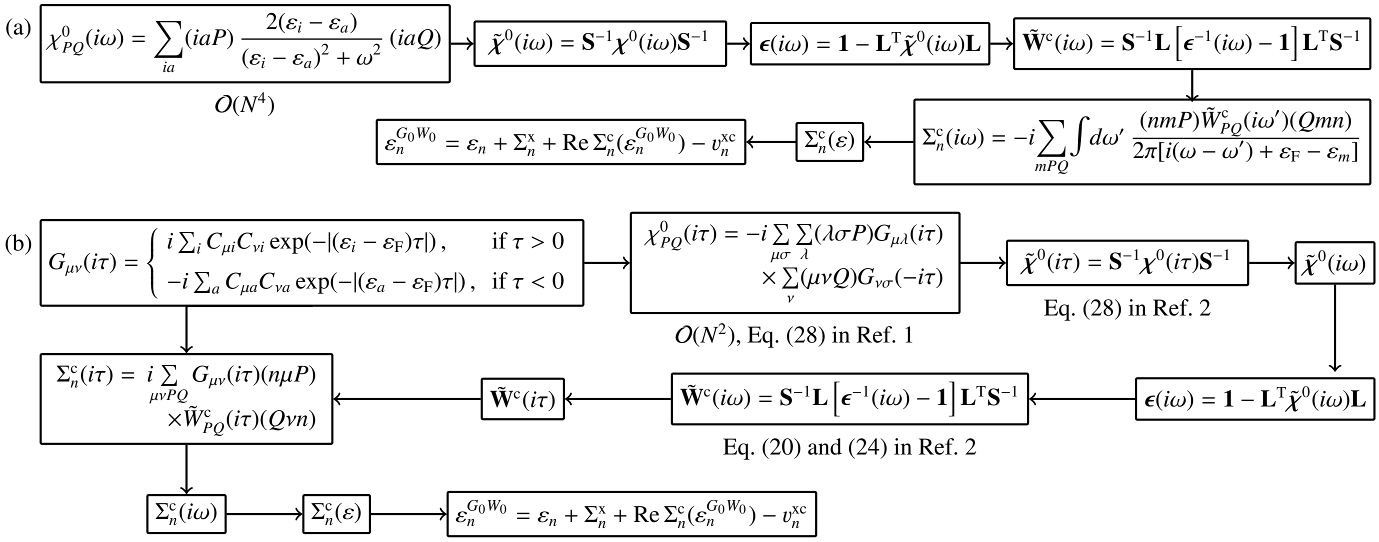


FIG. S1. Computational workflows of the canonical $O(N^4)$-scaling *GW* algorithm (a) from Ref. (3), and the low-scaling *GW* algorithm (b) based on the $O(N^3)$-scaling *GW* space-time method in a Gaussian basis. To simplify the comparison, both algorithms are sketched for resolution-of-the-identity (RI) with the overlap metric (4), despite algorithm (a) usually being paired with RI in the Coulomb metric.

## II. RESOLUTION OF THE IDENTITY

The occurance of three-center overlap tensors $(\nu\mu P)$ and the inverse of the overlap matrix $S_{PQ}$ can be derived from the resolution of the identity with the overlap metric (4–6) (RI-SVS)

$$(\mu\nu|\lambda\sigma)_{\text{RI-SVS}} = \sum_{PQRT} (\mu\nu P) S^{-1}_{PQ} V_{QR} S^{-1}_{RT} (T\lambda\sigma)\,. \tag{S1}$$

RI-SVS can be seen as twice inserting the identity operator $\mathrm{Id} = \sum_{PQ} |P\rangle\, S^{-1}_{PQ}\, \langle Q|$ into the left side of Eq. (S1) which is exact in the limit of a complete auxiliary basis $\{\varphi_P\}$. The sparsity of the three-center overlap integrals $(\mu\nu P)$ from Eq. (S1) is crucial to compute the polarizability in Eq. (3) from the main manuscript in $O(N^2)$ operations.

The popular RI with the Coulomb metric (RI-V), (4)

$$(\mu\nu|\lambda\sigma)_{\text{RI-V}} = \sum_{PQ} (\mu\nu|P) V^{-1}_{PQ} (Q|\lambda\sigma)\,, \tag{S2}$$

is commonly used in canonical $O(N^4)$-scaling *GW* implementations (3, 7, 8), since RI-V converges faster with the number $N_{\text{RI}}$ of RI basis functions. Due to the long-range nature of the Coulomb operator, however, the three-center Coulomb integrals $(\mu\nu|P)$ are not sparse in $\mu/P$ and $\nu/P$. This leads to a $O(N^4)$-scaling computation of $\chi^0_{PQ}(i\tau)$ in RI-V, (4), which is no advantage over canonical *GW*.

The overhead associated with increasing the RI basis, as required by RI-SVS, can be assessed by noting that the computational cost of both the low-scaling and $O(N^4)$ algorithms scales with $N^2_{\text{RI}}$. Increasing $N_{\text{RI}}$ for the low-scaling algorithm by a factor of $c \geq 1$ thus leads to an increase in computational cost by $c^2$. The system size $N$, at which the low-scaling algorithm becomes superior, increases, but only by a factor of $c$ – assuming $\approx N^2$ scaling for the low-scaling algorithm as in the example of graphene nanoribbons from Fig. (2) of the main manuscript.

## III. *GW*100 BENCHMARK

TABLE S1. $G_0W_0$@PBE HOMO and LUMO values for the *GW*100 (9) benchmark set obtained from the cubic-scaling *GW* algorithm as presented in the main manuscript using an analytic continuation with a Pade approximant. AIMS values marked with † are calculated using a 128 parameter Pade fit.

| Molecule (9) | HOMO FHI-aims 16-pole (9) | HOMO CP2K $O(N^3)$ code | LUMO FHI-aims 16-pole (9) | LUMO CP2K $O(N^3)$ code |
|---|---|---|---|---|
| 1 (helium, He) | −23.48 | −23.67 | 11.01 | 11.03 |
| 2 (neon, Ne) | −20.38 | −22.58 | 11.64 | 11.79 |
| 3 (argon, Ar) | −15.13 | −15.16 | 8.11 | 8.11 |
| 4 (krypton, Kr) | −13.57 | −13.57 | 7.63 | 7.57 |
| 5 (xenon, Xe) | −12.02 | −11.99 | 7.98 | 7.88 |
| 6 (hydrogen, $H_2$) | −15.81 | −15.78 | 3.50 | 3.49 |
| 7 (lithium dimer, $Li_2$) | −4.99 | −4.94 | −0.63 | −0.67 |
| 8 (sodium dimer, $Na_2$) | −4.83 | −4.81 | −0.55 | −0.57 |
| 9 (sodium tetramer, $Na_4$) | −4.10 | −4.09 | −1.01 | −1.03 |
| 10 (sodium hexamer, $Na_6$) | −4.24 | −4.23 | −0.97 | −0.96 |
| 11 (potassium dimer, $K_2$) | −3.98 | −3.98 | −0.65 | −0.66 |
| 12 (rubidium dimer, $Rb_2$) | −3.80 | −3.81 | −0.62 | −0.65 |
| 13 (nitrogen, $N_2$) | −14.89 | −14.92 | 2.45 | 2.48 |
| 14 (phosphorus dimer, $P_2$) | −10.21 | −10.26 | −0.72 | −0.71 |
| 15 (arsenic dimer, $As_2$) | −9.47 | −9.45 | −0.85 | −0.87 |
| 16 (fluorine, $F_2$) | −14.96 | −14.91 | −0.70 | −0.77 |
| 17 (chlorine, $Cl_2$) | −11.10 | −11.09 | −0.89 | −0.87 |
| 18 (bromine, $Br_2$) | −10.22 | −10.21 | −1.40 | −1.35 |
| 19 (iodine, $I_2$) | −9.28 | −9.28 | −1.68 | −1.68 |
| 20 (methane, $CH_4$) | −13.93 | −13.95 | 2.45 | 2.48 |
| 21 (ethane, $C_2H_6$) | −12.37 | −12.36 | 2.29 | 2.31 |
| 22 (propane $C_3H_8$) | −11.79 | −11.79 | 2.19 | 2.21 |
| 23 (butane, $C_4H_10$) | −11.49 | −11.49 | 2.14 | 2.16 |
| 24 (ethylene, $C_2H_4$) | −10.33 | −10.36 | 2.02 | 2.00 |
| 25 (ethyn, $C_2H_2$) | −11.02 | −11.07 | 2.86 | 2.87 |
| 26 (etracarbon, $C_4$) | −10.78 | −10.79 | −2.94 | −2.94 |
| 27 (cyclopropane, $C_3H_6$) | −10.56 | −10.56 | 2.45 | 2.47 |
| 28 (benzene, $C_6H_6$) | −8.99 | −9.00 | 1.09 | 1.06 |
| 29 (cyclooctatetraene, $C_8H_8$) | −8.06 | −8.02 | 0.06 | 0.03 |
| 30 (cyclopentadiene, $C_5H_6$) | −8.35 | −8.36 | 1.04 | 1.03 |
| 31 (vinyl fluoride, $C_2H_3F$) | −10.20 | −10.22 | 2.15 | 2.14 |
| 32 (vinyl chloride, $C_2H_3Cl$) | −9.76 | −9.78 | 1.42 | 1.41 |
| 33 (vinyl bromide, $C_2H_3Br$) | −8.99 | −8.99 | 1.38 | 1.37 |
| 34 (vinyl iodide, $C_2H_3I$) | −9.04 | −9.04 | 0.89 | 0.87 |
| 35 (tetrafluoromethane, $CF_4$) | −15.37 | −15.36 | 4.41 | 4.42 |
| 36 (tetrachloromethane, $CCl_4$) | −10.98 | −10.93 | −0.01 | −0.06 |
| 37 (tetrafbromomethane, $CBr_4$) | −9.90 | −9.91 | −1.08 | −1.08 |
| 38 (tetraiodomethane, $CI_4$) | −8.82 | −8.85 | −2.14 | −2.14 |
| 39 (silane, $SiH_4$) | −12.31 | −12.33 | 2.51 | 2.48 |
| 40 (germane, $GeH_4$) | −12.02 | −12.04 | 2.30 | 2.29 |
| 41 (disilane, $Si_2H_6$) | −10.31 | −10.29 | 1.69 | 1.65 |
| 42 (pentasilane, $Si_5H_{12}$) | −8.94 | −8.89 | 0.16 | 0.17 |
| 43 (lithium hydride, LiH) | −6.54 | −6.68 | −0.07 | −0.08 |
| 44 (potassium hydride, KH) | −4.86 | −5.56 | −0.18 | −0.23 |
| 45 (borane, $BH_3$) | −12.87 | −12.87 | 0.12 | 0.10 |
| 46 (diborane, $B_2H_6$) | −11.84 | −11.82 | 0.84 | 0.82 |
| 47 (ammonia, $NH_3$) | −10.32 | −10.28 | 2.31 | 2.33 |
| 48 (hydrozoic acid, $HN_3$) | −10.39 | −10.39 | 1.40 | 1.39 |
| 49 (phosphine, $PH_3$) | −10.27 | −10.27 | 2.50 | 2.47 |

TABLE S2. Continuation of Table S1.

| Molecule (9) | HOMO FHI-aims 16-pole (9) | HOMO CP2K $O(N^3)$ code | LUMO FHI-aims 16-pole (9) | LUMO CP2K $O(N^3)$ code |
|---|---|---|---|---|
| 50 (arsine, $AsH_3$) | −10.12 | −10.12 | 2.32 | 2.30 |
| 51 (hydrogen sulfide, $SH_2$) | −10.03 | −10.02 | 2.56 | 2.53 |
| 52 (hydrogen fluoride, HF) | −15.30 | −15.28 | 2.54 | 2.54 |
| 53 (hydrogen chloride, HCl) | −12.25 | −12.24 | 2.06 | 2.06 |
| 54 (lithium fluoride, LiF) | −9.95 | −9.77 | 0.09 | 0.09 |
| 55 (magnesium fluoride, $MgF_2$) | −12.32 | −12.23 | −0.14 | −0.15 |
| 56 (titanium tetrafluoride, $TiF_4$) | −13.89 | −13.92 | −0.60 | −0.60 |
| 57 (aluminium fluoride, $AlF_3$) | −14.25 | −14.29 | 0.16 | 0.14 |
| 58 (boron monofluoride, BF) | −10.56 | −10.63 | 1.22 | 1.21 |
| 59 (sulfur tetrafluoride, $SF_4$) | −12.12 | −12.10 | 0.38 | 0.36 |
| 60 (potassium bromide, BrK) | −7.30 | −7.58 | −0.31 | −0.31 |
| 61 (gallium monochloride, GaCl) | −9.55 | −9.58 | −0.02 | −0.03 |
| 62 (sodium chloride, NaCl) | −8.10 | −8.31 | −0.39 | −0.40 |
| 63 (magnesium chloride, $MgCl_2$) | −10.99 | −10.98 | −0.43 | −0.44 |
| 64 (aluminium iodide, $AlI_3$) | −9.32 | −9.34 | −0.80 | −0.82 |
| 65 (boron nitride, BN) | −11.03† | −11.13 | −3.88 | −3.87 |
| 66 (hydrogen cyanide, HCN) | −13.21 | −13.21 | 2.58 | 2.57 |
| 67 (phosphorus mononitride, PN) | −11.14 | −11.18 | −0.20 | −0.19 |
| 68 (hydrazine, $H2NNH_2$) | −9.28 | −9.23 | 1.99 | 2.00 |
| 69 (formaldehyde, $H_2CO$) | −10.33 | −10.31 | 0.96 | 0.93 |
| 70 (methanol, $CH_4O$) | −10.56 | −10.56 | 2.25 | 2.27 |
| 71 (ethanol, $C_2H_6O$) | −10.16 | −10.13 | 2.08 | 2.09 |
| 72 (acetaldehyde, $C_2H_4O$) | −9.55 | −9.54 | 1.05 | 1.03 |
| 73 (ethoxy ethane, $C_4H_{10}O$) | −9.32 | −9.29 | 2.10 | 2.12 |
| 74 (formic acid, $CH_2O_2$) | −10.73 | −10.73 | 1.91 | 1.90 |
| 75 (hydrogen peroxide, HOOH) | −10.99 | −11.00 | 2.35 | 2.33 |
| 76 (water, $H_2O$) | −11.97 | −11.95 | 2.37 | 2.38 |
| 77 (carbon dioxide, $CO_2$) | −13.25 | −13.26 | 2.50 | 2.50 |
| 78 (carbon disulfide, $CS_2$) | −9.75 | −9.78 | −0.20 | −0.20 |
| 79 (carbon oxide sulfide, COS) | −10.91 | −10.91 | 1.21 | 1.21 |
| 80 (carbon oxide selenide, COSe) | −10.20 | −10.21 | 0.87 | 0.87 |
| 81 (carbon monoxide, CO) | −13.57 | −13.58 | 0.67 | 0.67 |
| 82 (ozone, $O_3$) | −11.39† | −11.79 | −2.30 | −2.34 |
| 83 (sulfur dioxide, $SO_2$) | −11.82 | −11.84 | −1.00 | −1.00 |
| 84 (beryllium monoxide, BeO) | −8.58† | −9.20 | −2.56 | −2.27 |
| 85 (magnesium monoxide, MgO) | −6.68† | −6.70 | −1.89 | −1.90 |
| 86 (toluene, $C_7H_8$) | −8.61 | −8.63 | 1.01 | 0.99 |
| 87 (ethylbenzene, $C_8H_{10}$) | −8.55 | −8.57 | 1.04 | 1.02 |
| 88 (hexafluorobenzene, $C_6F_6$) | −9.49 | −9.47 | 0.66 | 0.63 |
| 89 (phenol, $C_6H_5OH$) | −8.37 | −8.36 | 0.96 | 0.94 |
| 90 (aniline, $C_6H_5NH_2$) | −7.64 | −7.63 | 1.15 | 1.12 |
| 91 (pyridine, $C_5H_5N$) | −9.04 | −9.01 | 0.51 | 0.49 |
| 92 (guanine, $C_5H_5N_5O$) | −7.69 | −7.70 | 0.74 | 0.74 |
| 93 (adenine, $C_5H_5N_5$) | −7.98 | −7.96 | 0.47 | 0.45 |
| 94 (cytosine, $C_4H_5N_3O$) | −8.29 | −8.27 | 0.26 | 0.25 |
| 95 (thymine, $C_5H_6N_2O_2$) | −8.71 | −8.71 | 0.06 | 0.05 |
| 96 (uracil, $C_4H_4N_2O_2$) | −9.22 | −9.20 | 0.01 | 0.00 |
| 97 (urea, $CH_4N_2O$) | −9.32 | −9.29 | 1.62 | 1.65 |
| 98 (silver dimer, $Ag_2$) | −7.07 | −6.98 | −1.05 | −0.92 |
| 99 (copper dimer, $Cu_2$) | −7.55 | −7.55 | −0.92 | −0.90 |
| 100 (copper cynide, CuCN) | −9.42† | −9.75 | −1.84 | −1.65 |

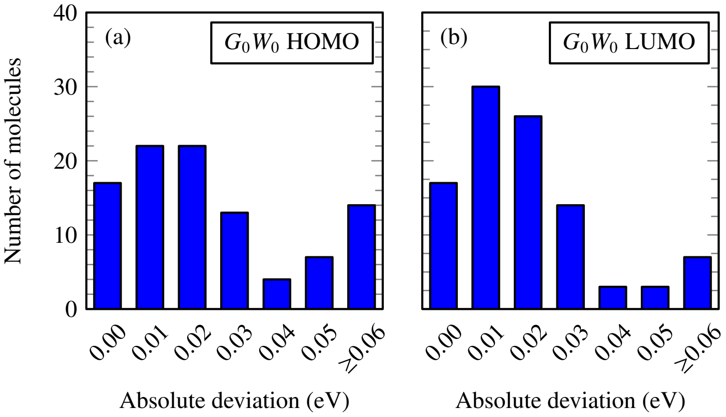


FIG. S2. Summary of the $GW100$ benchmark. Shown is the absolute deviation of $G_0W_0$@PBE (a) HOMO energies (ionization potentials) and (b) LUMO energies (electron affinities) from FHI-aims reference values (9).

## IV. OUTLIERS IN THE $GW100$ TEST SET

As stated in the main manuscript, we find a mean absolute deviation of 35 meV between FHI-aims (9) and our algorithm for the ionization potential, when excluding BN, $O_3$, BeO, MgO, CuCN and Ne from the $GW100$ test set. In the original $GW100$ benchmark (9), it was found that for $O_3$, BeO, and MgO, a Padé fit with 16 parameters was sufficient, while for BN and CNCu it was necessary to increase the number of parameters to 128 in order to describe the poles of the self-energy sufficiently accurately.

Since we employ minimax grids for imaginary time and frequency, which are restricted to at most 20 points, it is difficult for us to converge the pole structure of the molecules listed above. This has also been observed in the $GW100$ benchmark run using the low-scaling $GW$ algorithm in VASP (10, 11), where BN, $O_3$, BeO, MgO and CuCN also have been excluded from the $GW100$ test.

## V. CHOOSING THE FILTER THRESHOLD

The polarizability and the self-energy in Eqs. (3) and (10) of the manuscript are computed using sparse tensor operations. In particular, atomic blocks in the three-center overlap tensors are neglected, if their Frobenius norm falls below a given filter threshold. This threshold is a convergence parameter that needs to be chosen to achieve the desired accuracy of the calculation.

For the one-dimensional graphene nanoribbons under study, both computing time and accuracy vary slowly with the filter threshold. Table S3 illustrates this for the case of 6-anthene, i.e. the nanoribbon depicted in Fig. 3 (a) of the manuscript. Decreasing the filter threshold by a factor of 10 increases the computing time by less than 10 %, since the overlap of Gaussian basis functions located on different atoms decreases faster than exponentially with their distance.

We note that for too high filter thresholds $> 10^{-10}$, the dielectric function is no longer positive definite and thus its inversion by Cholesky decomposition is no longer possible.

TABLE S3. Converging the filter threshold for 6-anthene (114 atoms). Shown are the $G_0W_0$@PBE HOMO-LUMO gap and the execution time on 576 CPUs on a Cray XC40 machine as a function of the filter threshold for the three-center overlap integrals of Eq. (4). The augmented correlation-consistent double-$\zeta$ basis set together with the RI basis from the main manuscript has been used.

| Filter threshold | $G_0W_0$@PBE HOMO-LUMO gap (eV) | Fraction of unfiltered $(\mu\nu P)$ integrals | Execution time (s) |
|---|---|---|---|
| $10^{-10}$ | 2.485 | $5.0 \cdot 10^{-2}$ | 1296 |
| $10^{-11}$ | 2.433 | $5.8 \cdot 10^{-2}$ | 1485 |
| $10^{-12}$ | 2.435 | $6.7 \cdot 10^{-2}$ | 1561 |
| $10^{-13}$ | 2.434 | $7.5 \cdot 10^{-2}$ | 1720 |
| $10^{-14}$ | 2.434 | $8.2 \cdot 10^{-2}$ | 1843 |

## VI. EXEMPLARY CP2K INPUT FILE

We give the input file for the $G_0W_0$@PBE calculation for the GNR with 1734 atoms from the main manuscript.

```
&GLOBAL
  PROJECT  Cubic_GW_nanoribbon
  PRINT_LEVEL MEDIUM
  RUN_TYPE ENERGY
  EXTENDED_FFT_LENGTHS
&END GLOBAL
&FORCE_EVAL
  METHOD Quickstep
  &DFT
    BASIS_SET_FILE_NAME ./BASIS ! aug-DZVP basis from Ref. 3
    POTENTIAL_FILE_NAME POTENTIAL
    UKS
    MULTIPLICITY 1
    &MGRID
      CUTOFF 800
      REL_CUTOFF 60
    &END MGRID
    &QS
      METHOD GPW
      EPS_DEFAULT 1.0E-15
      EPS_PGF_ORB 1.0E-200
    &END QS
    ! For systems with dipoles / charges use POISSON_SOLVER MT
    &SCF
      EPS_SCF 1.0E-6
      MAX_SCF 15
      &OT
        MINIMIZER       CG
        PRECONDITIONER  FULL_SINGLE_INVERSE
      &END
      &OUTER_SCF
        EPS_SCF  1.0E-6
        MAX_SCF  5
      &END
      CHOLESKY OFF
      EPS_EIGVAL 1.0E-4
    &END SCF
    &XC
      &XC_FUNCTIONAL PBE
      &END XC_FUNCTIONAL
      &WF_CORRELATION
        METHOD RI_RPA_GPW
        RI OVERLAP
        ERI_METHOD OS
        &WFC_GPW
          ! EPS_FILTER controls the accuracy and the
          ! time for the cubic_scaling GW calculation
          EPS_FILTER  1.0E-9
          EPS_GRID 1.0E-6
          EPS_PGF_ORB_S 1.0E-20
        &END
        &RI_RPA
          RPA_NUM_QUAD_POINTS  12
          MINIMAX
          IM_TIME
          &IM_TIME
            EPS_FILTER_IM_TIME 1.0E-11
            GROUP_SIZE_3C 9
            GROUP_SIZE_P 1
            MEMORY_CUT  12
            GW
            MEMORY_INFO
          &END
          &RI_G0W0
            FIT_ERROR
            CORR_OCC 15
            CORR_VIRT 15
            CROSSING_SEARCH NEWTON
            CHECK_FIT
            EV_SC_ITER 1
            OMEGA_MAX_FIT 1.0
            ANALYTIC_CONTINUATION PADE
            RI OVERLAP
            RI_SIGMA_X
            PRINT_GW_DETAILS
          &END RI_G0W0
        &END RI_RPA
      &END
    &END XC
  &END DFT
                    ⋮
  &SUBSYS
    &CELL
      ABC [angstrom]  440.0  22.0  12.0
      ! this controls computation of overlap integrals in DFT/GW
      ! and Coulomb integrals in GW
      PERIODIC NONE
    &END CELL
    &KIND H
      BASIS_SET aug-DZVP-GTH
      RI_AUX_BASIS_SET RI_aug_DZ
      POTENTIAL  GTH-PBE-q1
    &END KIND
    &KIND C
      BASIS_SET  aug-DZVP-GTH
      RI_AUX_BASIS_SET RI_aug_DZ
      POTENTIAL  GTH-PBE-q4
    &END KIND
    &KIND C1 ! Breaking spin-up/spin-down symmetry on
      ! specific atoms in order to find correct spin state
      ELEMENT C
      BASIS_SET aug-DZVP-GTH
      RI_AUX_BASIS_SET RI_aug_DZ
      POTENTIAL GTH-PBE-q4
      &BS
        &ALPHA
          NEL 1
          L   1
          N   2
        &END
        &BETA
          NEL -1
          L   1
          N   2
        &END
      &END
    &END KIND
    &KIND C2
      ELEMENT C
      BASIS_SET aug-DZVP-GTH
      RI_AUX_BASIS_SET RI_aug_DZ
      POTENTIAL GTH-PBE-q4
      &BS
        &ALPHA
          NEL -1
          L   1
          N   2
        &END
        &BETA
          NEL 1
          L   1
          N   2
        &END
      &END
    &END KIND
    &TOPOLOGY
      COORD_FILE_NAME  ./struc.xyz
      COORD_FILE_FORMAT xyz
      &CENTER_COORDINATES
      &END
      ! generate reorder to preserve spin symmetry breaking
      &GENERATE
       REORDER
      &END GENERATE
    &END TOPOLOGY
  &END SUBSYS
&END FORCE_EVAL
```

## VII. BASIS SETS FOR GNR BENCHMARKS

The *GW* calculations on GNRs shown in Fig. 2 and 3 of the main manuscript use the aug-DZVP and the corresponding RI basis sets given below. These basis sets have been optimized for use with Goedecker-Teter-Hutter pseudopotentials (12).

Hydrogen aug-DZVP

| Shell Type | Exponents | Contraction Coefficients |
|---|---|---|
| *s* | 8.374435 | -0.028338 |
| | 1.805868 | -0.133381 |
| | 0.485252 | -0.399567 |
| *s* | 0.3220000 | 1.000000 |
| *s* | 0.1597400 | 1.000000 |
| *p* | 0.7270000 | 1.000000 |
| *p* | 0.2410000 | 1.000000 |

Hydrogen RI-aug-DZVP

| Shell Type | Exponents | Contraction Coefficients |
|---|---|---|
| *s* | 0.266913 | 1.000000 |
| *s* | 0.675611 | 1.000000 |
| *s* | 2.389278 | 1.000000 |
| *s* | 13.672245 | 1.000000 |
| *p* | 0.423431 | 1.000000 |
| *p* | 1.129610 | 1.000000 |
| *p* | 6.514017 | 1.000000 |
| *d* | 0.968755 | 1.000000 |

Carbon aug-DZVP

| Shell Type | Exponents | Contraction Coefficients |
|---|---|---|
| *s* | 4.336237 | 0.149079 |
| | 1.288183 | -0.029264 |
| | 0.403776 | -0.688204 |
| *s* | 0.279600 | 1.000000 |
| *s* | 0.136900 | 1.000000 |
| *p* | 4.336237 | -0.087812 |
| | 1.288183 | -0.277556 |
| | 0.403776 | -0.471229 |
| *p* | 0.151700 | 1.000000 |
| *p* | 0.110410 | 1.000000 |
| *d* | 0.650000 | 1.000000 |
| *d* | 0.171000 | 1.000000 |

Carbon RI-aug-DZVP

| Shell Type | Exponents | Contraction Coefficients |
|---|---|---|
| *s* | 0.189725 | 1.000000 |
| *s* | 0.367457 | 1.000000 |
| *s* | 0.609648 | 1.000000 |
| *s* | 1.389982 | 1.000000 |
| *s* | 3.169357 | 1.000000 |
| *s* | 7.226141 | 1.000000 |
| *p* | 0.162163 | 1.000000 |
| *p* | 0.377576 | 1.000000 |
| *p* | 0.925772 | 1.000000 |
| *p* | 2.525672 | 1.000000 |
| *p* | 7.212489 | 1.000000 |
| *d* | 0.116106 | 1.000000 |
| *d* | 0.487640 | 1.000000 |
| *d* | 0.983281 | 1.000000 |
| *d* | 6.201798 | 1.000000 |
| *f* | 0.270499 | 1.000000 |
| *f* | 1.142327 | 1.000000 |

Table S4 compares the HOMO-LUMO (zigzag) gap and the HOMO-1–LUMO+1 (transport) gap of 6-anthene, as computed with the aug-DZVP and the aug-TZVP basis. While the HOMO-LUMO gap between end-localized states is already converged to 10 meV, the HOMO-1–LUMO-1 gap between delocalized states still changes by 110 meV. For the purposes of the benchmark, these accuracies were deemed acceptable given the substantial difference in execution time.

TABLE S4. Dependence of $G_0W_0$@PBE energy gaps on the basis set. The aug-DZVP basis (+ corresponding RI basis) is listed above. The aug-TZVP basis (+ corresponding RI basis) was taken from the EMSL database, exponents below 0.09 were set to 0.09 to ensure good convergence of the SCF, and exponents above 20.0 were removed, since we use pseudopotentials (12) rather than treating core electrons explicitly.

| Basis set | $G_0W_0$@PBE HOMO-LUMO gap (eV) | $G_0W_0$@PBE HOMO-1–LUMO+1 gap (eV) | Execution time (CPU hours) |
|---|---|---|---|
| aug-DZVP | 2.43 | 3.87 | 238 |
| aug-TZVP | 2.42 | 3.98 | 3540 |

## VIII. REFERENCES

* jan.wilhelm@basf.com, Present address: BASF SE, Carl-Bosch-Straße 38, D-67056 Ludwigshafen am Rhein, Germany
† carlo.pignedoli@empa.ch

[1] Wilhelm, J.; Seewald, P.; Del Ben, M.; Hutter, J. Large-Scale Cubic-Scaling Random Phase Approximation Correlation Energy Calculations Using a Gaussian Basis. *J. Chem. Theory Comput.* **2016**, *12*, 5851–5859.
[2] Wilhelm, J.; Hutter, J. Periodic *GW* calculations in the Gaussian and plane-waves scheme. *Phys. Rev. B* **2017**, *95*, 235123.
[3] Wilhelm, J.; Del Ben, M.; Hutter, J. GW in the Gaussian and Plane Waves Scheme with Application to Linear Acenes. *J. Chem. Theory Comput.* **2016**, *12*, 3623–3635.
[4] Vahtras, O.; Almlöf, J.; Feyereisen, M. Integral approximations for LCAO-SCF calculations. *Chem. Phys. Lett.* **1993**, *213*, 514–518.
[5] Schurkus, H. F.; Ochsenfeld, C. Communication: An effective linear-scaling atomic-orbital reformulation of the random-phase approximation using a contracted double-Laplace transformation. *J. Chem. Phys.* **2016**, *144*, 031101.
[6] Duchemin, I.; Li, J.; Blase, X. Hybrid and Constrained Resolution-of-Identity Techniques for Coulomb Integrals. *J. Chem. Theory Comput.* **2017**, *13*, 1199–1208.
[7] Ren, X.; Rinke, P.; Blum, V.; Wieferink, J.; Tkatchenko, A.; Sanfilippo, A.; Reuter, K.; Scheffler, M. Resolution-of-identity approach to Hartree-Fock, hybrid density functionals, RPA, MP2 and GW with numeric atom-centered orbital basis functions. *New J. Phys.* **2012**, *14*, 053020.
[8] Blase, X.; Attaccalite, C.; Olevano, V. First-principles *GW* calculations for fullerenes, porphyrins, phtalocyanine, and other molecules of interest for organic photovoltaic applications. *Phys. Rev. B* **2011**, *83*, 115103.
[9] van Setten, M. J.; Caruso, F.; Sharifzadeh, S.; Ren, X.; Scheffler, M.; Liu, F.; Lischner, J.; Lin, L.; Deslippe, J. R.; Louie, S. G. et al. *GW*100: Benchmarking $G_0W_0$ for Molecular Systems. *J. Chem. Theory Comput.* **2015**, *11*, 5665–5687.
[10] Maggio, E.; Liu, P.; van Setten, M. J.; Kresse, G. GW100: A Plane Wave Perspective for Small Molecules. *J. Chem. Theory Comput.* **2017**, *13*, 635–648.
[11] Liu, P.; Kaltak, M.; Klimeš, J.; Kresse, G. Cubic scaling *GW*: Towards fast quasiparticle calculations. *Phys. Rev. B* **2016**, *94*, 165109.
[12] Goedecker, S.; Teter, M.; Hutter, J. Separable dual-space Gaussian pseudopotentials. *Phys. Rev. B* **1996**, *54*, 1703.
